# Supplementary material for: Finding Minimum Connected Subgraphs with Ontology Exploration on Large RDF Data
Source: arXiv:2010.06336 source file (2020-10-14)
Supplement: Supplementary file 1 [file appendix.tex]

\appendix
